# Supplementary material for: Molecular Mechanism of Gas Solubility in Liquid: Constant Chemical Potential Molecular Dynamics Simulations
Source: arXiv:2005.02770 source file (2020-05-06)
Supplement: Supplementary file 1 [file SI_Solubility_r.pdf]

# Supporting Information: Molecular Mechanism of Gas Solubility in Liquid: Constant Chemical Potential Molecular Dynamics Simulations

Narjes Ansari,[†,‡] Tarak Karmakar,[†,‡] and Michele Parrinello[*,†,‡,¶]

[†]†*Department of Chemistry and Applied Biosciences, ETH Zürich*

‡*Facoltà di informatica, Istituto di Scienze Computazionali, Università della Svizzera Italiana, CH-6900 Lugano, Switzerland*

¶*Italian Institute of Technology, Via Morego 30, 16163 Genova, Italy*

E-mail: parrinello@phys.chem.ethz.ch

# I: NPT simulations

Fig. S1 panel (a) shows a snapshot of the $CO_2$ - $H_2O$ simulation box of size ∼50 × 50 × 200 Å at the initial step. After around 100 ps, $CO_2$ molecules collapse in a layered structure (see panel (b)) of Fig. S1). In order to avoid such an artifact, we need to use a larger simulation box. For example for $CO_2$ - $H_2O$ system at T=323 K and P=50 bar, one needs to use a simulation box with a size of ∼50 × 50 × 400 Å. The situation is even worse for low-pressure cases. A simulation at T=323 K and P=1 bar demands even larger box, (∼1400 Å) along the z-axis to tackle large box fluctuations that arise due to the high compressibility of the gas.

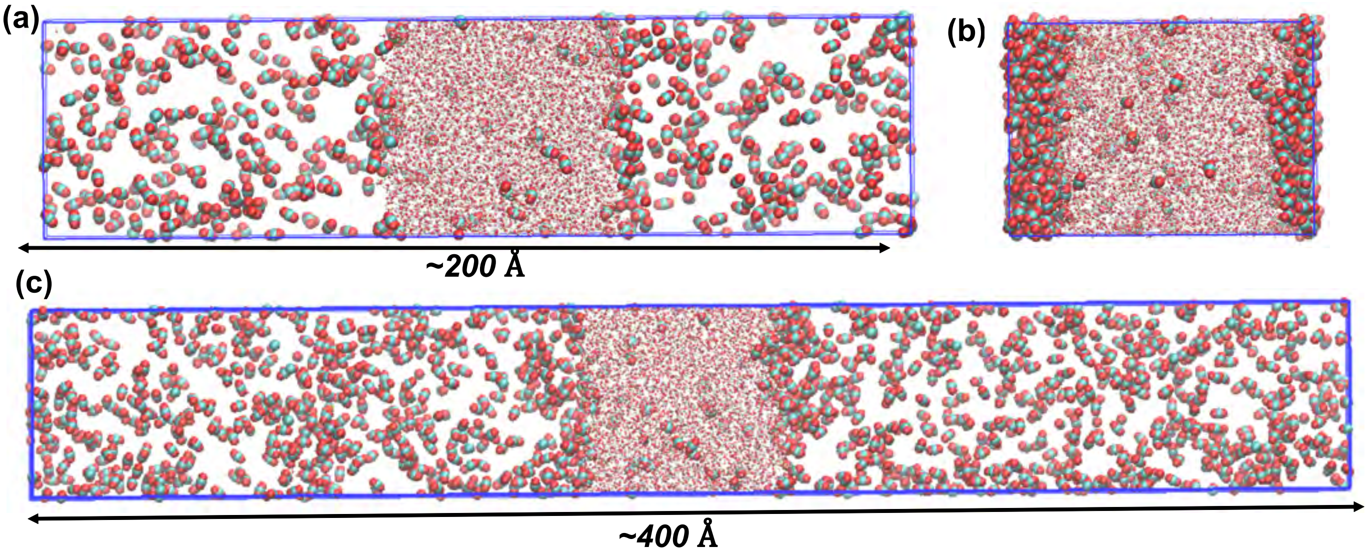


Figure S1: A snapshot of the $CO_2$ - $H_2O$ simulation box at a) t=0 ps and b) t=100 ps, c) larger simulation box.

# II: C$\mu$MD simulations parameters

In Table S1, we report the pre-equilibrated simulation box size, the $CO_2$ number density that we used for NVT-MD and C$\mu$MD simulations at (T=323 K, P=50 bar) and (T=423 K, P=100 bar).

Table S1: Cell parameter (a in Å) of a pre-equilibrated water slab, experimental density of $CO_2$ gas ($\rho_{CO_2}$ in kg/cm$^3$ collected from the National Institute of Standards and Technology-NIST[?] ), number of $CO_2$ molecules for NVT-MD simulations (N$_{CO_2}$ -MD), number of $CO_2$ molecules for C$\mu$MD simulations (N$_{CO_2}$ -C$\mu$MD), pressure (P) is in bar unit. Note that in the C$\mu$MD simulations, the reservoir contains more $CO_2$ molecules.

| **P (bar), T (K)** | **a** | $\rho_{CO_2}$ | **N$_{CO_2}$-NVT** | **N$_{CO_2}$ - C$\mu$MD** |
|---|---|---|---|---|
| 50, 323 | 50.17 | 104.85 | 544 | 708 |
| 100, 423 | 52.10 | 145.56 | 845 | 1000 |

Table S2 shows all the parameters, the length of the CR, TR, FR, and $\kappa$, required to carry out the C$\mu$MD simulations (see the main text for the description of these parameters).

Table S2: Parameters for C$\mu$MD simulations

| **P (bar), T (K)** | **CR (Å)** | **DCR (Å)** | **FR (Å)** | **k** |
|---|---|---|---|---|
| 50, 323 | 25 | 50 | 3 | 1000 |
| 100, 423 | 25 | 50 | 3 | 1000 |

Fig. S2 shows the density profile of $CO_2$ at T=323 K and P=50 bar obtained from the NVT-MD and C$\mu$MD simulations. At this thermodynamic condition, there is ~18 % depletion of $CO_2$ density in the gas phase of the NVT simulation, which is corrected in C$\mu$MD simulation (see solid line in Fig. S2).

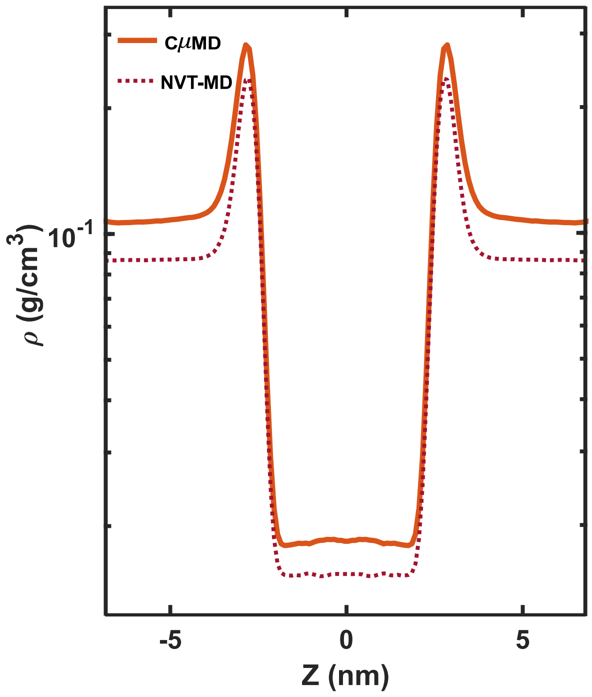


Figure S2: The density profile of $CO_2$ calculated from NVT-MD and C$\mu$MD simulations at T=323 K and P=50 bar (the y-axis is in log scale)

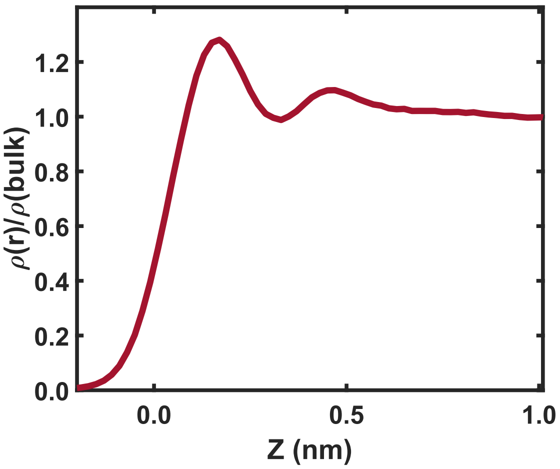


Figure S3: Time-averaged water density in the vicinity of the instantaneous surface normalized with respect to bulk liquid water at T=323 K and P=50 bar.

## III: Classification of the crest and trough molecules

As we mentioned in the main text, for identification of the crest and trough water molecules we used all water molecules ($W_{int}$) that are in the vicinity of the first layer of the interface. Panel (a) of Fig. S4 shows a snapshot of a WC interface and interfacial water molecules, $W_{int}$. First, we calculate the XY-plane distance $d_{O-WC}$ between oxygen atoms of $W_{int}$ and the grid points of the crest and trough regions. Since the maximum distance between two nearest neighbor grid points of WC is $\sim$ 2.4 Å, we assigned label crest to those $W_{int}$ with $d_{O-Crest} < 1.1$ Å(see panel (b) of Fig. S4) and trough to those with $d_{O-trough} < 1.1$ Å (see panel (c) of Fig. S4).

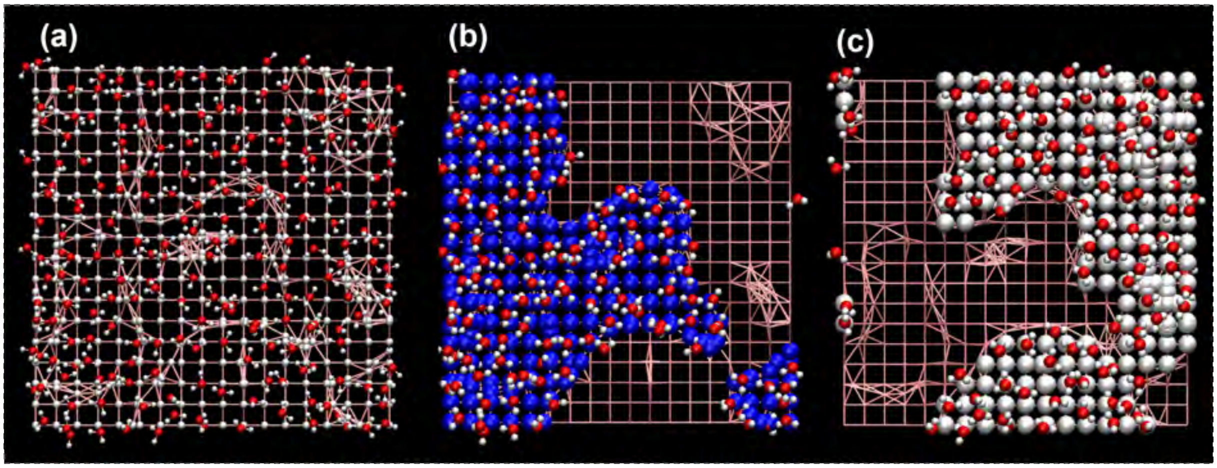


Figure S4: a) The WC interface (network frame) with $W_{int}$ in he vicinity the interface, (b) $W_{int}$ that belong to the crest, and (c) trough regions.

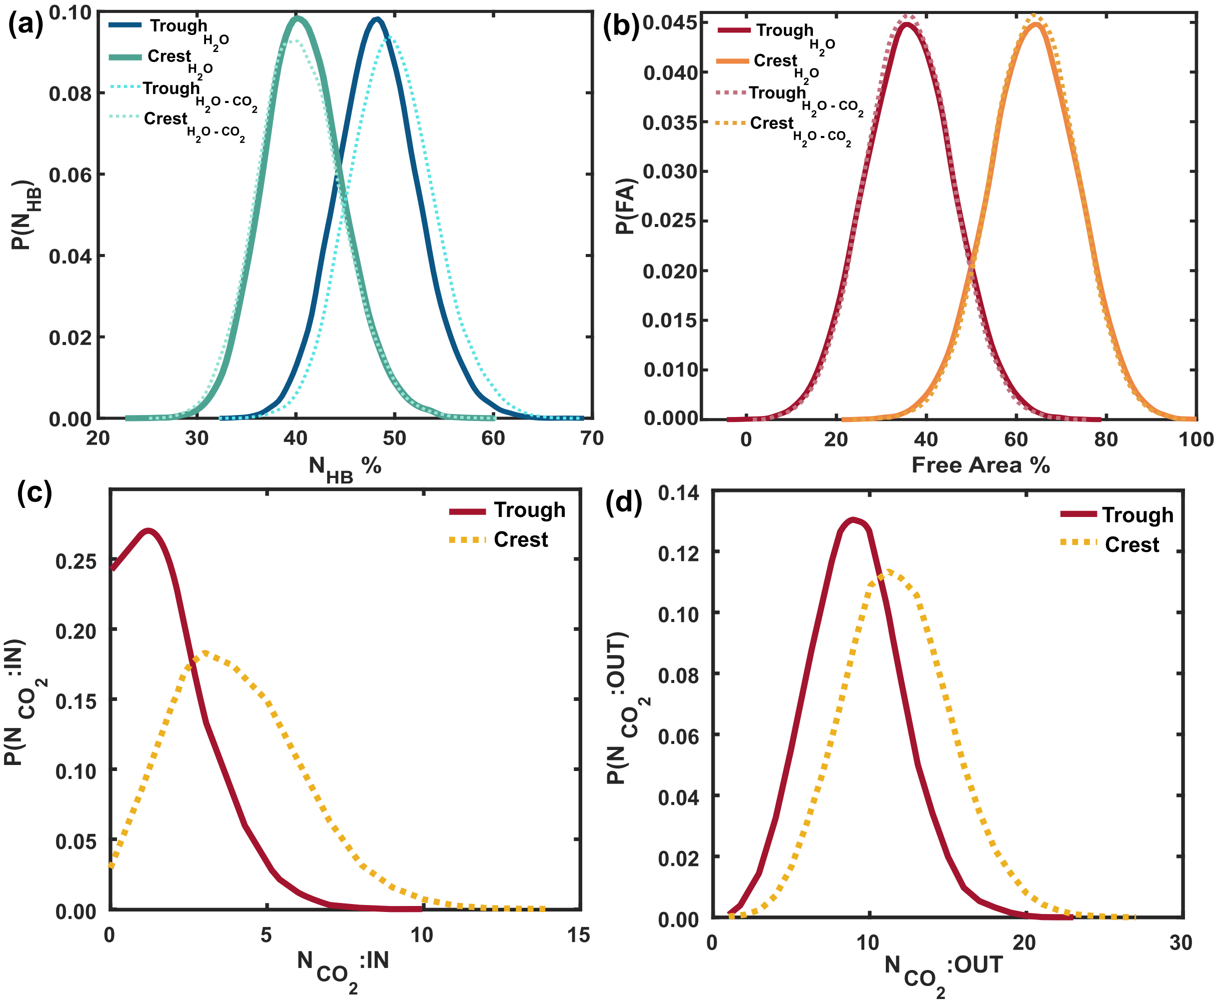


Figure S5: Percentage of hydrogen bonds that are under crest and trough regions within the first layer of water near the interface in both pure water-vapor and $CO_2$-$H_2O$ system, (b) the percentage of free area available under the crest and trough regions, (c) number of $CO_2$ molecules ($N_{CO_2}$:IN) within 2 Å of the crest and trough from the liquid side of the instantaneous interface, and (d) same as panel (c) from the gas side of the interface ($N_{CO_2}$:OUT). Here the densities of vapor $CO_2$ and liquid water are at T=323 K and P=50 bar.

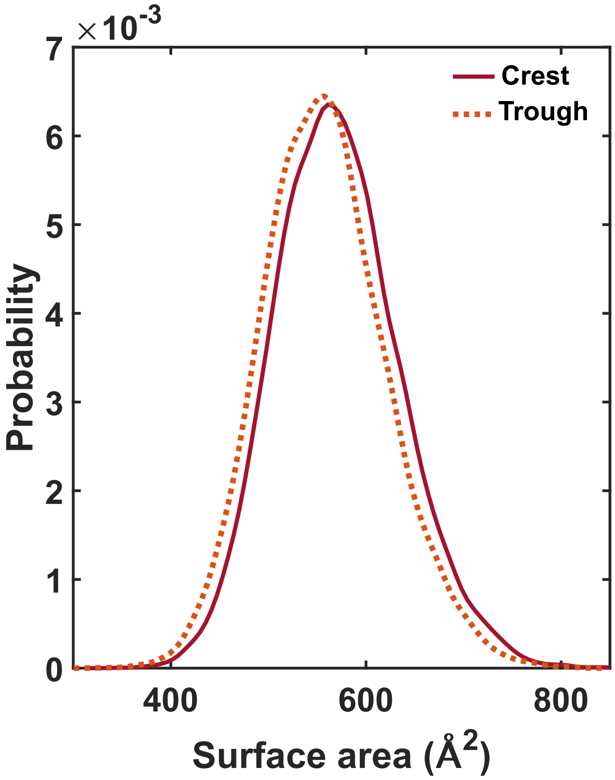


Figure S6: Surface area distribution of the crest and trough regions at T=323 K and P=50 bar.
